# Supplementary material for: Complementarity-constrained predictive control for efficient gas-balanced hybrid power systems
Source: arXiv:2404.06813 source file (2024-04-10)
Supplement: Supplementary file 1 [file appendix.tex]

\section{Look-up table approximations}\label{app:poly}

\subsection{Polynomial approximation of $C_\text{wtg}$}\label{subsec:polyapprox}

$C_\text{wtg}$ is the lookup table function for the aerodynamics of the wind turbines from \cite{Windtool} and is in this article approximated as a third order polynomial depending on the wind turbine blade pitch $\beta_\text{wtg}$ [deg] and the wind turbine tip speed ratio $\lambda_\text{wtg}$ [\si{\radian\per\second}] according to \cite{TORDMSC} (see equation \ref{eq:polyapproxs}),

\begin{align}
\label{eq:polyapproxs}
\begin{split}
     C_\text{wtg} = p_\text{wtg,00} &+ p_\text{wtg,{10}}\lambda_\text{wtg} + p_\text{wtg,{01}} \beta_\text{wtg}  \\&+ p_\text{wtg,{20}} \lambda_\text{wtg}^2+ p_\text{wtg,{11}} \lambda_\text{wtg} \beta_\text{wtg} \\&+ p_\text{wtg,{02}} \beta_\text{wtg}^2+ p_\text{wtg,{21}} \lambda_\text{wtg}^2\\
    &+ p_\text{wtg,{12}} \lambda_\text{wtg} \beta_\text{wtg}^2 + p_\text{wtg,{03}} \beta_\text{wtg}^3
\end{split}
\end{align}

where $p_\text{wtg,ij}$ are regression parameters and $\lambda_\text{wtg}$ is defined according to equation \ref{eq:wtg_turbine2}. The resulting approximations have an average mean squared error of 0.0020 for different average wind speeds $v_\text{wind}$ [\si{\metre\per\second}] (see table \ref{tab:Testpoly}). 

\begin{table}[ht]
	\centering
	\begin{tabular}{p{0.6cm} p{0.5cm} p{0.7cm} p{0.7cm} p{0.7cm} p{0.7cm} p{0.7cm} p{0.8cm}}
		{\textbf{Deg $\beta_\text{wtg}$}}& {\textbf{Deg $\lambda_\text{wtg}$}} & {\textbf{$v_\text{wind}$ = $1$}} & {\textbf{$v_\text{wind}$ = $6$}} &
		{\textbf{$v_\text{wind}$ = $11$}} &
		{\textbf{$v_\text{wind}$ = $16$}} &
		{\textbf{$v_\text{wind}$ = $21$}} &
		{\textbf{AMSE}}\\
		\hline
		
		$1$ & $2$ & $0.0107$ & $0.0056$ & $0.0016$ & $0.0004$ & $0.0011$ & $0.0039$ \\ \hline
		$1$ & $3$ & $0.0058$ & $0.0035$ & $0.0013$ & $0.0006$ & $0.0012$ & $0.0025$ \\ \hline
		$2$ & $2$ & $0.0107$ & $0.0056$ & $0.0016$ & $0.0004$ & $0.0011$ & $0.0039$ \\ \hline
		$2$ & $3$ & $0.0045$ & $0.0033$ & $0.0037$ & $0.0049$ & $0.0051$ & $0.0043$ \\ \hline
		$3$ & $2$ & $0.0050$ & $0.0023$ & $0.008$ & $0.0007$ & $0.0010$ & $0.0020$ \\ \hline
		$3$ & $3$ & $0.0070$ & $0.0061$ & $0.0070$ & $0.0085$ & $0.0086$ & $0.0074$ \\ \hline
	\end{tabular}
	\caption{Average mean square error for different degrees of the wind turbine blade pitch $\beta_\text{wtg}$ [deg] and the wind turbine tip rotational speed $\lambda_\text{wtg}$ [\si{\radian\per\second}] for different average wind speeds $v_\text{wind}$ [\si{\metre\per\second}].}
	\label{tab:Testpoly}
\end{table} 

\subsection{Sigmoidal approximation of $D_\text{wtg}$}\label{subsec:sigmoidapprox}

\cite{Windtool} defines the generator torque $D_\text{wtg}$ [$\si{\newton\metre}$] as an function of $\omega_\text{wtg}$ [\si{\radian\per\second}] and power demand reference given by a generator torque controller. To simplify, \cite{TORDMSC} approximates the generator torque controller with a look-up table, dependent only on $\omega_\text{wtg}$. Additionally, \cite{TORDMSC} provides a continuous approximation of the look-up table which is used in this paper for describing $D_\text{wtg}$ in both the plant and the control model (see equation \ref{eq:Dwgtg}),

\begin{equation}
     D_\text{wtg} =  \frac{M_\text{wtg,{gen,{max}}}}{1 + e^{-K_\text{wtg}(\omega_\text{{wtg,gen}} - K_\text{wtg,$\omega$})}}\label{eq:Dwgtg}
\end{equation}

where $M_\text{wtg,{gen,{max}}}$ [$\si{\newton\metre}$] is the maximum torque, $K_\text{wtg,{gen}}$ is a constant to adjust the curve steepness, and $\omega_\text{wtg,{gen,{mid}}}$ [$\si{\radian\per\second}$] is the midpoint of the functions slope. The resulting approximation have a R-square value of $0.99$ compared to the initial look-up table approximation.

\section{Model and Control parameters}\label{app:modelpara}

\begin{table}[ht!]
	\centering
	\begin{tabular}{p{3cm} p{1cm} p{1.5cm} p{1.5cm}}
		{\textbf{Parameter}}& {\textbf{Value}} & {\textbf{Unit}}& {\textbf{Symbol}} \\
		\hline
		Time constants &  $0.5$ & \si{\second} & $\tau_\text{gtg,V}$\\
		&  $0.5$ & \si{\second} & $\tau_\text{gtg,P}$\\ \hline
		Power constraints &  $0$ & \si{\kilo\watt}  & $P_\text{gtg,{{{min}}}}$\\
		&  $4500$ & \si{\kilo\watt} & $P_\text{gtg,{{max}}}$\\
		\hline
		Initial conditions &  $0$ &  pu & $V_\text{0,gtg}$\\
		&  $0$ & $\si{\kilo\watt}$ & $P_\text{0,gtg}$\\
		\hline
	\end{tabular}
	\caption{Gas turbine generator parameters, adapted from \cite{GAST}}
	\label{tab:GTG-Parameters}
\end{table}

\begin{table}[ht!]
	\centering
	\begin{tabular}{p{2.7cm}p{1.5cm}p{1.2cm}p{1.3cm}}
	{\textbf{Parameter}}& {\textbf{Value}} & {\textbf{Unit}}& {\textbf{Symbol}} \\
		\hline
		Rotor disk area &  $12468.98$ & \si{\metre\squared} & $A_\text{wtg}$\\ \hline
		Blade radius &  $63$ & \si{\metre} & $R_\text{wtg}$\\ \hline
		Gear ratio &  $97$ &  & $N_\text{wtg}$\\ \hline
		Inertia of turbine &  $35444067$ & \si{\kg\metre\squared} & $I_\text{wtg}$ \\ \hline
		Inertia of generator &  $534.116$ & \si{\kg\metre\squared} & $I_{\omega_\text{wtg,gen}}$ \\ \hline
		Generator time constant &  $0.5$ & \si{\second} & $\tau_\text{wtg}$ \\ 
		\hline
		Power constraints &  $0$ & \si{\kilo\watt}  & $P_\text{wtg,{{{min}}}}$\\
		&  $4500$ & \si{\kilo\watt} & $P_\text{wtg,{{max}}}$\\
		\hline
		Initial conditions &  $0.9$ &  \si{\radian\per\second} & $\omega_\text{0,wtg}$\\
		&  $0$ &  \si{\N\metre} & $M_\text{0,wtg,gen}$\\
		\hline
	\end{tabular}
	\caption{Wind turbine generator parameters, adapted from \cite{Windtool}}
	\label{tab:WTG-Parameters}
\end{table}

\begin{table}[!ht]
	\centering
	\begin{tabular}{p{3cm}p{1.2cm}p{1.3cm}p{1.2cm}}
		{\textbf{Parameter}}& {\textbf{Value}} & {\textbf{Unit}}& {\textbf{Symbol}} \\
		\hline
		Battery storage capacity&  $6.5$ & \si{\A\hour}& $Q_\text{bat}$\\
		\hline
		Constant potential&  $1.28$      &\si{\V}& $E_\text{bat,0}$\\
		\hline
		Internal resistance&  $2$        &  \si{\milli\ohm} &$R_\text{bat,{i}}$\\
		\hline
		Polarisation constant&  $9.1$    & \si{\milli\V} & $K_\text{bat}$\\
		\hline
		Exponential zone amplitude&  $111$& \si{\milli\V} & $A_\text{bat}$ \\
		\hline
		Exponential zone time constant inverse&  $2.31$ &\si{\per\A\per\hour} & $B_\text{bat}$ \\
		\hline
		Packs per battery&  $421$ &- &$\eta_\text{{packs}}$\\
		\hline
		Cells per pack&  $626$ & -&$\eta_\text{{bat,cells}}$\\
		\hline
		Power constraints &  $-4500$ & \si{\kilo\watt}  & $P_\text{bat,{{{min}}}}$\\
		&  $4500$ & \si{\kilo\watt} & $P_\text{bat,{{max}}}$\\
		\hline
		SOC constraints &  $0$ & \%  & $\text{SOC}_\text{bat,{{{min}}}}$\\
		&  $1$ & \% & $\text{SOC}_\text{bat,{{max}}}$\\
		\hline
	\end{tabular}
	\caption{Battery parameters, adapted from \cite{tremblay}}
	\label{tab:bat-Parameters}
\end{table}

\begin{table}[ht!]
	\centering
	\begin{tabular}{p{2cm}p{2cm}p{1cm}p{1.7cm}}
		{\textbf{Parameter}}& {\textbf{Value}} & {\textbf{Unit}}& {\textbf{Symbol}} \\
		\hline
		Maximum generator torque & $45700$ & \si{\newton\metre} & $M_\text{wtg,{gen,{max}}}$ \\ \hline
		Exponential constant & $0.099$ &  & $K_\text{wtg}$\\ \hline
		Rotational speed constant & $97$ & \si{\radian\per\second} & $K_{\text{wtg},\omega}$\\ \hline
		Torque regression coefficients & $-0.118600000$ & & $p_\text{wtg,{00}}$\\
		& $0.128900000$ & & $p_\text{wtg,{10}}$\\
		& $0.009222000$ & & $p_\text{wtg,{01}}$\\
	    & $-0.006314000$ & & $p_\text{wtg,{20}}$\\
	    & $-0.005206000$ & & $p_\text{wtg,{11}}$\\
	    & $-0.000159800$ & & $p_\text{wtg,{02}}$\\
	    & $-0.000102600$ & & $p_\text{wtg,{21}}$\\
	    & $0.000040100$ & & $p_\text{wtg,{12}}$\\
	    & $0.000000806$ & & $p_\text{wtg,{03}}$\\ \hline
	
	\end{tabular}
	\caption{Lookup table approximation parameters, refer to \cite{TORDMSC}}
	\label{tab:lookup-parameters}
\end{table}

\begin{table}[ht!]
	\centering
	\begin{tabular}{p{2.5cm}p{1cm}p{1.25cm}p{1.75cm}}
		{\textbf{Parameter}}& {\textbf{Value}} & {\textbf{Unit}}& {\textbf{Symbol}} \\
		\hline
	    State constraints 
		&  $1$ & pu & $V_\text{gtg,{{max}}}$\\
		&  $4500$ & \si{\kilo\watt} & $P_\text{gtg,{{max}}}$\\
		&  $inf$ & \si{\radian\per\second}& $\omega_\text{wtg,{{max}}}$\\
		&  $45700$ &  \si{\N\metre}  & $M_\text{wtg,gen,{{max}}}$\\
		&  $0$ & pu & $V_\text{gtg,{{min}}}$\\
		&  $100$ & \si{\kilo\watt} & $P_\text{gtg,{{min}}}$\\
		&  $0.001$ & \si{\radian\per\second} & $\omega_\text{wtg,{{min}}}$\\
		&  $0$ & \si{\N\metre} & $M_\text{wtg,gen,{{min}}}$\\\hline
		Input constraints 
		&  $1$ & pu & $T_\text{gtg,{{max}}}$\\
		&  $90$ & deg & $\beta_\text{wtg,{{max}}}$\\
		&  $200$ & \si{\A} & $I_\text{bat,{{max}}}$\\
		&  $0$ & pu & $T_\text{gtg,{{min}}}$\\
		&  $0$ & deg & $\beta_\text{wtg,{{min}}}$\\
		&  $-200$ & A & $I_\text{bat,{{min}}}$\\\hline
		Output constraints 
		&  $4500$ & \si{\kilo\watt} & $P_\text{gtg,{{max}}}$\\
		&  $4500$ & \si{\kilo\watt} & $P_\text{wtg,{{max}}}$\\
		&  $4500$ & \si{\kilo\watt} & $P_\text{bat,{{max}}}$\\
		&  $0$ & \si{\kilo\watt} & $P_\text{wtg,{{max}}}$\\
		&  $0$ & \si{\kilo\watt} & $P_\text{gtg,{{min}}}$\\
		&  $-4500$ & \si{\kilo\watt} & $P_\text{bat,{{min}}}$\\\hline
		SOC constraints &  $0.1$ & \%  & $\text{SOC}_\text{bat,{{{min}}}}$\\
		&  $1$ & \% & $\text{SOC}_\text{bat,{{max}}}$\\
		\hline
	\end{tabular}
	\caption{General Control parameters}
	\label{tab:General-Parameters}
\end{table}

\begin{table}[ht!]
	\centering
	\begin{tabular}{p{3cm}p{1.5cm}p{0.9cm}p{1.65cm}}
		{\textbf{Parameter}}& {\textbf{Value}} & {\textbf{Unit}}& {\textbf{Symbol}} \\
		\hline
		 Weighting constants &  $100$ &  & $K_\text{hlc,gtg}$\\
		 &  $-0.1$ & & $K_\text{hlc,wtg}$\\
		 &  $0.3$ & & $K_\text{hlc,bat}$\\
		 &  $100$ && $K_\text{hlc,u,1}$\\
		&  $200$ && $K_\text{hlc,u,2}$\\
		&  $8$ && $K_\text{hlc,u,3}$\\
		&  eye($nX+1$) &  & $K_\text{hlc,s}$\\
		\hline
		Sampling time & $3500$ & \si{\s} &$ t_\text{hlc,sampling}$\\\hline
		Prediction horizon & $7000$ & \si{\s} &$ t_\text{hlc,prediction}$\\\hline
		Control Horizon & $7000$ & \si{\s} &$ t_\text{hlc,control}$\\\hline
		Control Discretization & $14000$ &  &$ t_\text{hlc,discretization}$\\\hline
	\end{tabular}
	\caption{High-Level Control parameters}
	\label{tab:HLC-ENMPC-Parameters}
\end{table}

\begin{table}[ht!]
	\centering
	\begin{tabular}{p{3cm}p{1.5cm}p{0.9cm}p{1.65cm}}
		{\textbf{Parameter}}& {\textbf{Value}} & {\textbf{Unit}}& {\textbf{Symbol}} \\
		\hline
		 Weighting constants
		 &  $1$ && $K_\text{llc,x,1}$\\
		&  $0.01$ && $K_\text{llc,x,2}$\\
		&  $100$ && $K_\text{llc,x,3}$\\
		&  $0.00020$ && $K_\text{llc,x,4}$\\
		&  $1$ && $K_\text{llc,x,5}$\\
		&  $100$ && $K_\text{llc,u,1}$\\
		&  $100$ && $K_\text{llc,u,2}$\\
		&  $5$ && $K_\text{llc,u,3}$\\
		&  eye($nX+1$) &  & $K_\text{llc,s}$\\
		\hline
		Sampling time & $0.5$ & \si{\s} &$ t_\text{llc,sampling}$\\\hline
		Prediction horizon & $10$ & \si{\s} &$ t_\text{llc,prediction}$\\\hline
		Control Horizon & $10$ & \si{\s} &$ t_\text{llc,control}$\\\hline
		Control Discretization & $20$ &  &$ t_\text{llc,control}$\\\hline
	\end{tabular}
	\caption{Low-Level Control parameters}
	\label{tab:LLC-NMPC-Parameters}
\end{table} 
\clearpage
